# Supplementary material for: MATCHA:Towards Matching Anything
Source: arXiv:2501.14945 source file (2025-01-24)
Supplement: Supplementary file 1 [file suppmat.tex]

\documentclass[10pt,twocolumn,letterpaper]{article}

\usepackage[review]{cvpr}      %

\usepackage{arydshln}
\input{preamble}

\definecolor{cvprblue}{rgb}{0.21,0.49,0.74}
\usepackage[pagebackref,breaklinks,colorlinks,allcolors=cvprblue]{hyperref}

\title{Supplementary Material of MATCHA\includegraphics[scale=0.1]{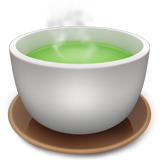}}

\author{First Author\\
Institution1\\
Institution1 address\\
{\tt\small firstauthor@i1.org}
\and
Second Author\\
Institution2\\
First line of institution2 address\\
{\tt\small secondauthor@i2.org}
}

\begin{document}
\maketitle

\input{sec/6_supplementary}

\clearpage

{
    \small
    \bibliographystyle{ieeenat_fullname}
    \bibliography{main}
}

\end{document}
